# Supplementary material for: Using Hindsight to Anchor Past Knowledge in Continual Learning
Source: arXiv:2002.08165 source file (2021-03-02)
Supplement: Supplementary file 1 [file appendix.pdf]

## Appendix

Section A describes the approximate update performed by anchoring objective (Eq. 5 in the main paper). Section B reports more experimental results. Section C provides the grid considered for hyper-parameters. Section E gives pseudo-code for HAL.

### A Approximate Update by Anchoring Objective

Here we will use a Taylor series expansion to approximate the update performed by anchoring objective (Eq. 5 in the main paper). In particular, we are interested in the regularization part of the anchoring objective that involves nested update. We refer to this gradient as  $g_{\perp}$ . We follow similar arguments as [Nichol and Schulman 2018].

Let  $\theta_0$  be the parameter vector before the temporary update in the anchoring objective (Eq. 5). Also, let  $\ell_{ce}$  and  $\ell_{L2}$  be the cross-entropy and L2 losses, respectively. We use the following definitions:

$$\begin{aligned}\bar{g}_0 &= \ell'_{ce}(\theta_0) && \text{(gradient of cross-entropy loss at initial point on } \mathcal{B} \cup \mathcal{B}_{\mathcal{M}}) \\ \bar{H}_0 &= \ell''_{ce}(\theta_0) && \text{(Hessian of cross-entropy loss at initial point on } \mathcal{B} \cup \mathcal{B}_{\mathcal{M}}) \\ \bar{g}_1 &= \ell'_{L2}(\theta_0) && \text{(gradient of L2 loss at initial point on anchors)} \\ \bar{H}_1 &= \ell''_{L2}(\theta_0) && \text{(Hessian of L2 loss at initial point on anchors)}\end{aligned}$$

Let  $U_0 = \theta_0 - \alpha \bar{g}_0$  be the operator giving a temporary update in the two-step process of (Eq. 5), and let  $\theta_1$  be the temporary update itself (*i.e.*)  $\theta_1 := U_0$  (note that  $\theta$  is used in the main paper instead of  $\theta_1$ ). The  $g_{\perp}$  is given by:

$$\begin{aligned}g_{\perp} &= \frac{\partial}{\partial \theta_0} \ell_{L2}(U_0) \\ &= U'_0 \cdot \ell'_{L2}(\theta_1) \\ &= (I - \alpha \bar{H}_0) \cdot \ell'_{L2}(\theta_1),\end{aligned}\tag{10}$$

where the second step is obtained by using chain rule. Now, if we calculate the first order Taylor series approximation of  $\ell'_{L2}(\theta_1)$ ,

$$\begin{aligned}\ell'_{L2}(\theta_1) &= \ell'_{L2}(\theta_0) + \ell''_{L2}(\theta_0) \cdot (\theta_1 - \theta_0) + O(\|\theta_1 - \theta_0\|^2) \\ &= \bar{g}_1 + \bar{H}_1 \cdot (\theta_0 - \alpha \bar{g}_0 - \theta_0) + O(\alpha^2) \\ &= \bar{g}_1 - \alpha \bar{H}_1 \cdot \bar{g}_0 + O(\alpha^2),\end{aligned}\tag{11}$$

where in the second step we substituted the value of  $\theta_1$ . By putting Eq. 11 in Eq. 10 and after some simplification we get:

$$g_{\perp} = \bar{g}_1 - \alpha (\bar{H}_1 \cdot \bar{g}_0 + \bar{H}_0 \cdot \bar{g}_1) + O(\alpha^2).\tag{12}$$

This form is very similar to the second-order MAML gradient formulation, Eq. 25 in [Nichol and Schulman 2018]. Further simplification of the inner product terms between Hessian and gradients yields inner product between the gradients  $\bar{g}_0$  and  $\bar{g}_1$ . This shows that similar to MAML [Finn, Abbeel, and Levine 2017], Reptile [Nichol and Schulman 2018] and MER [Riemer et al. 2019], anchoring objective, as described in Eq. 5 of the main paper, maximizes the inner product between the gradients. However, unlike the other meta-learning approaches, in anchoring objective, these gradients correspond to different loss functions, cross-entropy and L2 losses on data from current task and episodic memory, and HAL anchors, respectively.

### B More Results

Figure 3 shows a more fine grained analysis of average accuracy as new tasks are learned on Permuted MNIST and Split CIFAR. HAL preserves the performance of a predictor more effectively than other baselines.

Tables 5 and 6 show the Accuracy and Forgetting of methods employing episodic memory when the size of memory is increased. We use 3 to 5 examples per class per task, resulting in a total memory size from 600 to 1000 for MNIST experiments, and from 255 to 425 for CIFAR and ImageNet experiments.

### C Hyper-parameter Selection

In this section, we report the hyper-parameters grid considered for experiments. The best values for different benchmarks are given in parenthesis.

- Multitask

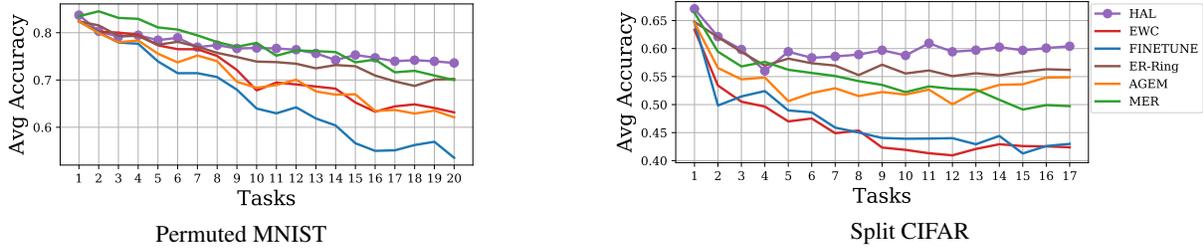

Figure 3: Evolution of Accuracy (Eq. 2) as new tasks are learned. When used, episodic memories contain up to one example per class per task.

Table 4: Impact of anchor selection, where we compare a randomly chosen data point as an anchor (Real Data Anchor) with our optimized anchor selection (HAL).

| Anchor type       | Split CIFAR                         |                                     |
|-------------------|-------------------------------------|-------------------------------------|
|                   | Accuracy                            | Forgetting                          |
| Real Data Anchor  | 58.0 ( $\pm 0.15$ )                 | 0.12 ( $\pm 0.01$ )                 |
| <b>HAL (ours)</b> | <b>60.4 (<math>\pm 0.54</math>)</b> | <b>0.10 (<math>\pm 0.01</math>)</b> |

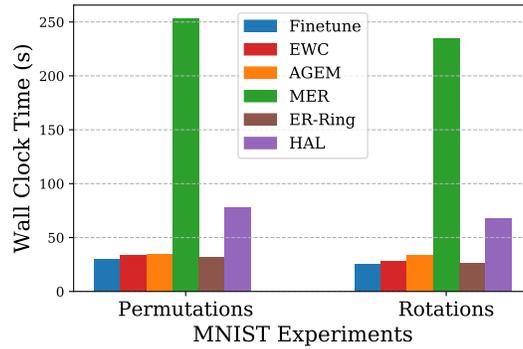

Figure 4: Training time (s) of MNIST experiments for the entire continual learning experience. MER and HAL both use meta-learning objectives to reduce forgetting.

- learning rate: [0.003, 0.01, 0.03 (CIFAR, miniImageNet), 0.1 (MNIST perm, rot), 0.3, 1.0]
- Clone-and-finetune
  - learning rate: [0.003, 0.01, 0.03 (CIFAR, miniImageNet), 0.1 (MNIST perm, rot), 0.3, 1.0]
- Finetune
  - learning rate: [0.003, 0.01, 0.03 (CIFAR, miniImageNet), 0.1 (MNIST perm, rot), 0.3, 1.0]
- EWC
  - learning rate: [0.003, 0.01, 0.03 (CIFAR, miniImageNet), 0.1 (MNIST perm, rot), 0.3, 1.0]
  - regularization: [0.1, 1, 10 (MNIST perm, rot, CIFAR, miniImageNet), 100, 1000]
- AGEM
  - learning rate: [0.003, 0.01, 0.03 (CIFAR, miniImageNet), 0.1 (MNIST perm, rot), 0.3, 1.0]
- MER

Table 5: Accuracy (Eq. 2) results for large (3 to 5 examples per class per task) episodic memory sizes. Here we only compare methods that use an episodic memory. Metrics are averaged over five runs using different random seeds.

| METHOD            | PERMUTED MNIST             |                            | ROTATED MNIST              |                            |
|-------------------|----------------------------|----------------------------|----------------------------|----------------------------|
|                   | $ \mathcal{M}  = 600$      | $ \mathcal{M}  = 1000$     | $ \mathcal{M}  = 600$      | $ \mathcal{M}  = 1000$     |
| VCL-RANDOM        | 55.8 ( $\pm 1.29$ )        | 58.5 ( $\pm 1.21$ )        | 61.2 ( $\pm 0.12$ )        | 64.4 ( $\pm 0.16$ )        |
| AGEM              | 63.2 ( $\pm 1.47$ )        | 64.1 ( $\pm 0.74$ )        | 49.9 ( $\pm 1.49$ )        | 53.0 ( $\pm 1.52$ )        |
| MER               | 74.9 ( $\pm 0.49$ )        | 78.3 ( $\pm 0.19$ )        | 76.5 ( $\pm 0.30$ )        | 77.3 ( $\pm 1.13$ )        |
| ER-RING           | 73.5 ( $\pm 0.43$ )        | 75.8 ( $\pm 0.24$ )        | 74.7 ( $\pm 0.56$ )        | 76.5 ( $\pm 0.48$ )        |
| <b>HAL (OURS)</b> | <b>76.2</b> ( $\pm 0.52$ ) | <b>78.4</b> ( $\pm 0.27$ ) | <b>77.0</b> ( $\pm 0.66$ ) | <b>78.7</b> ( $\pm 0.97$ ) |

  

| METHOD            | SPLIT CIFAR                |                            | SPLIT MINIIMAGENET         |                            |
|-------------------|----------------------------|----------------------------|----------------------------|----------------------------|
|                   | $ \mathcal{M}  = 255$      | $ \mathcal{M}  = 425$      | $ \mathcal{M}  = 255$      | $ \mathcal{M}  = 425$      |
| ICARL             | 51.7 ( $\pm 1.41$ )        | 51.2 ( $\pm 1.32$ )        | -                          | -                          |
| AGEM              | 56.9 ( $\pm 3.45$ )        | 59.9 ( $\pm 2.64$ )        | 51.6 ( $\pm 2.69$ )        | 54.3 ( $\pm 1.56$ )        |
| MER               | 57.7 ( $\pm 2.59$ )        | 60.6 ( $\pm 2.09$ )        | 49.4 ( $\pm 3.43$ )        | 54.8 ( $\pm 1.79$ )        |
| ER-RING           | 60.9 ( $\pm 1.44$ )        | 62.6 ( $\pm 1.77$ )        | 53.5 ( $\pm 1.42$ )        | 54.2 ( $\pm 3.23$ )        |
| <b>HAL (OURS)</b> | <b>62.9</b> ( $\pm 1.49$ ) | <b>64.4</b> ( $\pm 2.15$ ) | <b>56.5</b> ( $\pm 0.87$ ) | <b>57.2</b> ( $\pm 1.54$ ) |

Table 6: Forgetting (Eq. 3) results for large (3 to 5 examples per class per task) episodic memory sizes. Here we only compare methods that use an episodic memory. Averages and standard deviations are computed over five runs using different random seeds.

| METHOD            | PERMUTED MNIST             |                            | ROTATED MNIST              |                            |
|-------------------|----------------------------|----------------------------|----------------------------|----------------------------|
|                   | $ \mathcal{M}  = 600$      | $ \mathcal{M}  = 1000$     | $ \mathcal{M}  = 600$      | $ \mathcal{M}  = 1000$     |
| VCL-RANDOM        | 0.39 ( $\pm 0.01$ )        | 0.36 ( $\pm 0.01$ )        | 0.37 ( $\pm 0.01$ )        | 0.33 ( $\pm 0.01$ )        |
| AGEM              | 0.20 ( $\pm 0.01$ )        | 0.19 ( $\pm 0.01$ )        | 0.41 ( $\pm 0.01$ )        | 0.38 ( $\pm 0.01$ )        |
| MER               | 0.14 ( $\pm 0.01$ )        | 0.09 ( $\pm 0.01$ )        | <b>0.12</b> ( $\pm 0.01$ ) | <b>0.11</b> ( $\pm 0.01$ ) |
| ER-RING           | 0.09 ( $\pm 0.01$ )        | 0.07 ( $\pm 0.01$ )        | 0.15 ( $\pm 0.01$ )        | 0.13 ( $\pm 0.01$ )        |
| <b>HAL (OURS)</b> | <b>0.07</b> ( $\pm 0.01$ ) | <b>0.05</b> ( $\pm 0.01$ ) | <b>0.12</b> ( $\pm 0.01$ ) | <b>0.11</b> ( $\pm 0.01$ ) |

  

| METHOD            | SPLIT CIFAR                |                            | SPLIT MINIIMAGENET         |                            |
|-------------------|----------------------------|----------------------------|----------------------------|----------------------------|
|                   | $ \mathcal{M}  = 255$      | $ \mathcal{M}  = 425$      | $ \mathcal{M}  = 255$      | $ \mathcal{M}  = 425$      |
| ICARL             | 0.13 ( $\pm 0.02$ )        | 0.13 ( $\pm 0.02$ )        | -                          | -                          |
| AGEM              | 0.13 ( $\pm 0.03$ )        | 0.10 ( $\pm 0.02$ )        | 0.10 ( $\pm 0.02$ )        | 0.08 ( $\pm 0.01$ )        |
| MER               | 0.11 ( $\pm 0.01$ )        | 0.09 ( $\pm 0.02$ )        | 0.12 ( $\pm 0.02$ )        | 0.07 ( $\pm 0.01$ )        |
| ER-RING           | 0.09 ( $\pm 0.01$ )        | <b>0.06</b> ( $\pm 0.01$ ) | 0.07 ( $\pm 0.02$ )        | 0.08 ( $\pm 0.02$ )        |
| <b>HAL (OURS)</b> | <b>0.08</b> ( $\pm 0.01$ ) | <b>0.06</b> ( $\pm 0.01$ ) | <b>0.06</b> ( $\pm 0.01$ ) | <b>0.06</b> ( $\pm 0.01$ ) |

- learning rate: [0.003, 0.01, 0.03 (MNIST, CIFAR, miniImageNet), 0.1, 0.3, 1.0]
- within batch meta-learning rate: [0.01, 0.03, 0.1 (MNIST, CIFAR, miniImageNet), 0.3, 1.0]
- current batch learning rate multiplier: [1, 2, 5 (CIFAR, miniImageNet), 10 (MNIST)]
- ER-Ring
  - learning rate: [0.003, 0.01, 0.03 (CIFAR, miniImageNet), 0.1 (MNIST perm, rot), 0.3, 1.0]
- HAL
  - learning rate: [0.003, 0.01, 0.03 (CIFAR, miniImageNet), 0.1 (MNIST perm, rot), 0.3, 1.0]
  - regularization ( $\lambda$ ): [0.01, 0.03, 0.1 (MNIST perm, rot), 0.3 (miniImageNet), 1 (CIFAR), 3, 10]

- mean embedding strength ( $\gamma$ ): [0.01, 0.03, 0.1 (MNIST perm, rot, CIFAR, miniImageNet), 0.3, 1, 3, 10]
- decay rate ( $\beta$ ): 0.5
- gradient steps on anchors ( $k$ ): 100

## D Hyperparameter Sensitivity

In Table 7, we report the performance of HAL against a range of hyperparameters. For a given hyperparameter in the table, all the other hyperparameters are set to their optimal values found in Sec C of the appendix. HAL is not sensitive to the choice of hyperparameters.

Table 7: Average Accuracy of HAL on different values of hyperparameters. For a given hyperparameter in the table, all the other hyperparameters are set to their optimal values found in Sec C of the appendix.

| DATASET        | $\lambda$ | ACC               | $\gamma$ | ACC               | $\beta$ | ACC               |
|----------------|-----------|-------------------|----------|-------------------|---------|-------------------|
| PERMUTED MNIST | 0.01      | 72.8 $\pm$ (0.52) | 0.01     | 73.1 $\pm$ (0.20) | 0.1     | 72.5 $\pm$ (0.95) |
|                | 0.1       | 73.6 $\pm$ (0.31) | 0.1      | 73.6 $\pm$ (0.31) | 0.5     | 73.6 $\pm$ (0.31) |
|                | 1.0       | 73.2 $\pm$ (0.85) | 1.0      | 73.4 $\pm$ (0.41) | 0.9     | 72.9 $\pm$ (0.39) |
| SPLIT CIFAR100 | 0.01      | 58.5 $\pm$ (1.25) | 0.01     | 59.8 $\pm$ (0.65) | 0.1     | 58.7 $\pm$ (1.17) |
|                | 0.1       | 59.2 $\pm$ (0.91) | 0.1      | 60.4 $\pm$ (0.54) | 0.5     | 60.4 $\pm$ (0.54) |
|                | 1.0       | 60.4 $\pm$ (0.54) | 1.0      | 60.2 $\pm$ (1.21) | 0.9     | 59.6 $\pm$ (1.05) |

## E HAL Algorithm

Algorithm 1 provides pseudo-code for HAL.

**Algorithm 1** Training of HAL on sequential data  $\mathcal{D} = \{\mathcal{D}_1, \dots, \mathcal{D}_T\}$ , with total replay buffer size ‘mem\_sz’, learning rate ‘ $\alpha$ ’, regularization strength ‘ $\lambda$ ’, mean embedding decay ‘ $\beta$ ’, mean embedding strength ‘ $\eta$ ’.

---

```

1: procedure HAL( $\mathcal{D}$ , mem_sz,  $\alpha$ ,  $\lambda$ ,  $\beta$ )
2:    $\mathcal{M} \leftarrow \{\}$  * mem_sz
3:    $\{e_1, \dots, e_T\} \leftarrow \{\}$ 
4:   for  $t \in \{1, \dots, T\}$  do
5:      $\phi_t \leftarrow \vec{0}$ 
6:     for  $\mathcal{B} \sim \mathcal{D}_t$  do
7:        $\mathcal{B}_{\mathcal{M}} \sim \mathcal{M}$ 
8:        $\theta \leftarrow \theta - \alpha \cdot \nabla_{\theta} \ell(\mathcal{B} \cup \mathcal{B}_{\mathcal{M}})$ 
9:        $\theta \leftarrow \theta - \alpha \cdot \nabla_{\theta} \left( \ell(\mathcal{B} \cup \mathcal{B}_{\mathcal{M}}) + \lambda \cdot \sum_{t' < t} (f_{\theta}(e_{t'}, t') - f_{\bar{\theta}}(e_{t'}, t'))^2 \right)$ 
10:       $\phi_t \leftarrow \beta \cdot \phi_t + (1 - \beta) \cdot \phi(\mathcal{B})$ 
11:       $\mathcal{M} \leftarrow \text{UpdateMemory}(\mathcal{M}, \mathcal{B})$ 
12:    end for
13:     $e_t, \theta \leftarrow \text{GetAnchors}(\mathcal{M}, \theta, \phi_t, \eta)$ 
14:  end for
15:  return  $\theta, \mathcal{M}$ 
16: end procedure

1: procedure GETANCHORS( $\mathcal{M}, \theta_t, \phi_t, \gamma$ )
2:    $\theta \leftarrow \theta_t$ 
3:   for  $\mathcal{B}_{\mathcal{M}} \sim \mathcal{M}$  do
4:      $\theta \leftarrow \theta - \alpha \cdot \nabla_{\theta} \ell(\mathcal{B}_{\mathcal{M}})$ 
5:   end for
6:    $\theta_{\mathcal{M}} \leftarrow \theta$ 
7:    $e_t \leftarrow \text{rand}()$ 
8:   for  $1, \dots, k$  do
9:      $e_t \leftarrow e_t + \alpha \cdot \nabla_{e_t} \left( \ell(f_{\theta_{\mathcal{M}}}(e_t, t), y_t) - \ell(f_{\theta_t}(e_t, t), y_t) - \gamma(\phi(e_t) - \phi_t)^2 \right)$ 
10:  end for
11:  return  $e_t, \theta_t$ 
12: end procedure

```

---

▷ Sample a batch from current task  
 ▷ Sample a batch from episodic memory  
 ▷ Temporary parameter update  
 ▷ Anchoring objective (Eq. 5)  
 ▷ Running average of mean embedding  
 ▷ Add samples to a ring buffer  
 ▷ Get anchors for current task  
 ▷ Finetune  $\theta_t$  by taking SGD steps on the episodic memory  
 ▷ Store the updated parameter  
 ▷ Initialize the task anchors  
 ▷ Maximize forgetting (Eq. 9)
